# Supplementary material for: Learning to Unlearn: Instance-wise Unlearning for Pre-trained Classifiers
Source: arXiv:2301.11578 source file (2024-01-15)
Supplement: Supplementary file 1 [file supple_table.tex]

% \begin{table}[!t]
%          \caption{Correcting adversarial images from ImageNet-A. \textsc{Adv} achieves the least forgetting, while \textsc{Adv+Imp} fails to correct large number of predictions due to strong regularization.}
%         \label{table:imagenet_a_results}
%         \vspace{-.1in}  
%         \centering
%         \footnotesize
%         \smallskip\noindent
%         \resizebox{\linewidth}{!}{
%         \begin{tabular}{ll|ccccccc}
%             \toprule
%             &  & \multicolumn{4}{c}{ImageNet-A}\\ 
%             &  & {$k=16$} & {$k=32$} & {$k=64$} & $k=128$ & $k=256$ & $k=512$ & $k=1024$\\ 
%             \midrule
%             \multirow{4}{*}{$D_f$ ($\uparrow$)} 
%             & \textsc{Before}  & 0.0 & 0.0 & 0.0 & 0.0  & 0.20 & &\\ 
%             & \textsc{Correct}  & 100.0 & 100.0 & 100.0 & 100.0  & & &\\ 
%             & \textsc{Adv}  & 100.0 & 100.0 & 95.31 & 83.44  & 84.38 & &\\ 
%             & \textsc{Adv+Imp}  & 100.0 & 100.0 & 10.94 & 9.38  & 6.64 & &\\  
%             \midrule
%             \multirow{4}{*}{$D_r$ ($\uparrow$)}  
%             & \textsc{Before}  & 87.46 & 87.46 & 87.46 & 87.46  & & &\\ 
%             & \textsc{Correct}  & \textbf{84.41} & 83.29 & 80.79 & 77.38  & & &\\ 
%             & \textsc{Adv}  & 81.75 & \textbf{83.80} & \textbf{83.74} & \textbf{83.44} & \textbf{83.29} & &\\ 
%             & \textsc{Adv+Imp}  & 81.82 & 83.73 & 83.53 & 82.86 & 80.56 & &\\ 
%             \midrule
%             \multirow{4}{*}{$D_{test}$ ($\uparrow$)} 
%             & \textsc{Before}  & 76.15 & 76.15 & 76.15 & 76.15 & & &\\ 
%             & \textsc{Correct}  & \textbf{73.21} & 72.04 & 69.91 & 66.73 & & &\\ 
%             & \textsc{Adv}  & 70.89 & \textbf{72.58} & \textbf{72.68} & \textbf{72.36} & \textbf{72.13}& &\\ 
%             & \textsc{Adv+Imp}  & 70.98 & 72.51 & 72.39& 71.68 & 69.30 & &\\ 
%             \bottomrule
%         \end{tabular}
%         }
% \end{table}
